# Supplementary material for: The Fusion of Large Language Models and Formal Methods for Trustworthy AI Agents: A Roadmap
Source: arXiv:2412.06512 source file (2024-12-09)
Supplement: Supplementary file 1 [file appendix.tex]

%%%%%%%%%%%%%%%%%%%%%%%%%%%%%%%%%%%%%%%%%%%%%%%%
\section{Appendix}\label{sec:app}
%%%%%%%%%%%%%%%%%%%%%%%%%%%%%%%%%%%%%%%%%%%%%%%%
